# Supplementary material for: A Comprehensive Evaluation of GPT-4V on Knowledge-Intensive Visual Question Answering
Source: arXiv:2311.07536 source file (2024-08-24)
Supplement: Supplementary file 1 [file appendix.tex]

\begin{table}[t]

\tabcolsep=0.11cm
  \caption{Model performances on VQA with commonsense knowledge. The knowledge scope contains Scene Understanding (SU), Instance Identity (II), Instance Location (IL), Instance Attribute (IA), Instance Counting (IC),  Spatial Relation (SR), Instance Interaction (IIR),  Visual Reasoning (VR), and Text Recognition (TR).}
  \label{seed-bench}
  \centering
  \scriptsize
  \begin{tabular}{l|cccccccccc}
    \toprule
    %\cmidrule(r){1-2}
    Models$\downarrow$ Types $\rightarrow$ & Overall  & SU & II & IL& IA&IC & SR & IIR& VR & TR\\
    \hline
    OpenFlamingo v2~\citep{alayrac2022flamingo} & 34.51 & 43.86	& 38.12 &	31.28&	30.06	& 27.30 & 30.59& 29.90& 50.15 & 20.00\\
    MiniGPT-4~\citep{zhu2023minigpt} &  47.40 & 56.27& 49.15&	45.82&	37.93	&45.32	&32.57	&47.42 &57.10 &11.76 \\
    MMGPT~\citep{mmgpt} &  34.54 & 43.64	&37.85	&31.45	& 30.78 &	27.34	&30.14	&29.90 & 51.36 & 18.82 \\
    BLIP-2 FlanT5-XL~\citep{li2023blip2}	& 49.74	&	59.12	& 53.90	&49.19	&42.33	&43.15	&36.68  &	55.67 & 45.62 & 25.88\\
    InstructBLIP FlanT5-XL~\citep{liu2023visual}	& 57.80	&	60.29	& 58.49	&63.37	&40.59	&58.44	&38.66&	51.55 &45.92 & 25.88 \\
    InstructBLIP Vicuna~\citep{liu2023visual}	& 58.76	&	60.20	&58.93	&\textbf{65.63}	&43.56	& \textbf{57.05}  &  40.33 &	52.58 & 47.73 & \textbf{43.53} \\
    LLaVA~\citep{liu2023visual} & 36.96 & 42.69 &	34.90&	33.45&	28.43&	41.85&	30.75&	27.84 &46.83 & 37.65\\
    LLaMA-Adapter-v2~\citep{gao2023llama}&	35.19&	45.22	&38.50	&29.30	&33.03 &	29.67	&35.46	&39.18 & 51.96&24.71\\
    GVT~\citep{GVT2023} & 35.49 & 41.74& 35.50& 31.79& 29.45& 36.17&31.96 & 31.96& 51.06&27.06\\
    VPGTrans~\citep{VPGTrans2023}& 41.81	&51.87	&44.13	&39.90	&36.09&	33.71	&36.38 & 31.96& 53.17 & 30.59\\
    mPLUG-Owl ~\citep{ye2023mplug} &	37.88	&	49.68	& 45.33 &	32.52	&36.71 &27.26	&32.72 &	44.33 &54.68 & 18.82\\
    Otter~\citep{li2023otter}	& 35.16	&	44.90	&38.56	&32.24&	30.88 &	26.28&31.81 & 31.96 &51.36 & 31.76\\
    
    LMEye (ours)	& \textbf{59.70} & \textbf{73.20} &  \textbf{64.12} & 56.57 & \textbf{53.99} &  48.75 & \textbf{47.64} & \textbf{65.98}& \textbf{76.13} & 37.65\\
    \bottomrule
  \end{tabular}
\end{table}
